# Supplementary material for: Efficient algorithms for optimal homology problems and their applications
Source: arXiv:2406.19422 source file (2024-06-26)
Supplement: Supplementary file 1 [file app.tex]

\appendix

%%%%%%%%%% DON'T DELETE THIS, REVERTS NUMBERING BACK %%%%%%%%%%%%%
\makeatletter
\renewcommand{\@makechapterhead}[1]{\vspace *{-10\p@ }{\parindent \z@ 
\raggedright \normalfont \ifnum \c@secnumdepth >\m@ne \Huge \bfseries 
\@chapapp \space \thechapter \vskip 10\p@ \fi #1\par \nobreak \vskip 30\p@ }}
\makeatother
%%%%%%%%%% DON'T DELETE THIS, REVERTS NUMBERING BACK %%%%%%%%%%%%%

\import{./}{appendix-fn-flow-examples}

%\chapter{MSFN: LP vs MinCostFlow}
%\vspace*{-0.3in}
%\begin{figure}[hb!]
%\begin{center}
%\makebox[\textwidth][c]{\includegraphics[width=1.0\textwidth]{figs/costperMb2015_4.jpg}}
%\end{center}
%\caption[Cost per raw megabase of DNA sequence from 2001 to 2015]{Cost per raw megabase of DNA sequence from 2001 to 2015. Straight line - Moore's Law, blue curve - cost in US dollars, Y-axis scale is logarithmic. Graph reproduced from \citep{wetterstrand2016}}
%\end{figure}

%\chapter{MSFN: Structural Validation Of Synthetic Power Distribution Networks}
%\begin{figure}[hb!]
%\begin{center}
%\includegraphics[scale=0.5]{figs/costperMb2015_4.jpg}
%\end{center}
%\caption[Cost per raw megabase of DNA sequence from 2001 to 2015]{Cost per raw megabase of DNA sequence from 2001 to 2015. Straight line - Moore's Law, blue curve - cost in US dollars, Y-axis scale is logarithmic. Graph reproduced from \citep{wetterstrand2016}}
%\end{figure}

\chapter{Persistent Cycles in Directed Bipartite Graph}

%\import{./}{appendix-react-plots.tex}

%\section{Examples: Super-Fast mechanism}
%\section{Analysis: Distance between persistence diagrams}
%\section{Analysis: Distribution of Cycle Representatives}
%
%\begin{figure}[hb!]
%\begin{center}
%\includegraphics[scale=0.5]{figs/costperMb2015_4.jpg}
%\end{center}
%\caption[Cost per raw megabase of DNA sequence from 2001 to 2015]{Cost per raw megabase of DNA sequence from 2001 to 2015. Straight line - Moore's Law, blue curve - cost in US dollars, Y-axis scale is logarithmic. Graph reproduced from \citep{wetterstrand2016}}
%\end{figure}

%\chapter{Other appendix}
%\begin{figure}[hb!]
%\begin{center}
%\includegraphics[scale=0.5]{figs/costperMb2015_4.jpg}
%\end{center}
%\caption[Cost per raw megabase of DNA sequence from 2001 to 2015]{Cost per raw megabase of DNA sequence from 2001 to 2015. Straight line - Moore's Law, blue curve - cost in US dollars, Y-axis scale is logarithmic. Graph reproduced from \citep{wetterstrand2016}}
%\end{figure}
